# Supplementary material for: Tensor Generalized Canonical Correlation Analysis
Source: arXiv:2302.05277 source file (2023-02-10)
Supplement: Supplementary file 2 [file B_old.tex]

\section{Proposition 1: Sketch of proof}
The proof of Proposition 1 directly follows the demonstration proposed in \citep{Tenenhaus2017}. It relies on two key ingredients: (i) the compactness of the feasible set $\Omega_l$ defined in Section 3.2 from the main text and (ii) the uniqueness of the update $\text{r}_l(\mathbf{w})$ defined in equation (7) in the main text.



\subsection{Compactness of the feasible set}
\label{compactness}

The proof of Proposition 1 relies on the compactness of $\Omega_l$ defined as:
\begin{equation}
\Omega_l = \{ \mathbf{w}_l \in \mathbb{R}^{p_l}; ~ \mathbf{w}_l = \sum_{r = 1}^{R_l} \lambda_l^{(r)} \mathbf{w}_l^{(r)}; ~ \mathbf{w}_l^{(r)} = \mathbf{w}_{l, d_l}^{(r)} \otimes \dots \otimes \mathbf{w}_{l,1}^{(r)}; ~ \mathbf{w}_l^{(r)\top} \mathbf{M}_l \mathbf{w}_l^{(s)} = \delta_{rs} ; ~ \boldsymbol{\lambda}_l^\top \boldsymbol{\lambda}_l = 1 \}  
\label{Omega}
\end{equation}
To show this result, we introduce the following sets:
\begin{align*}
    \Omega_\text{norm} &= \{ \mathbf{w}_l \in \mathbb{R}^{p_l}; \quad \mathbf{w}_l^\top \mathbf{M}_l \mathbf{w}_l = 1 \}, \\
    \Omega_\text{kron} &= \{ \mathbf{w}_l \in \mathbb{R}^{p_l}; \quad \mathbf{w}_l = \mathbf{w}_{l,d_l} \otimes \dots \otimes \mathbf{w}_{l,1} \}, \\
    \Omega_\text{mat} &= \{  \mathbf{W}_l \in \mathbb{R}^{p_l \times R_l}; \quad \mathbf{W}_l = \begin{bmatrix} \mathbf{w}_l^{(1)} & \dots & \mathbf{w}_l^{(R_l)} \end{bmatrix}; \quad \mathbf{w}_l^{(r)} \in \Omega_\text{norm} \cap \Omega_\text{kron} \}, \\
    \Omega_\text{orth} &= \{  \mathbf{W}_l \in \mathbb{R}^{p_l \times R_l}; \quad \mathbf{W}_l^\top \mathbf{M}_l \mathbf{W}_l = \mathbf{I}_{R_l} \}, \\
    \Lambda_l &= \{\boldsymbol{\lambda}_l \in \mathbb{R}^{R_l}; \quad \boldsymbol{\lambda}_l^\top \boldsymbol{\lambda}_l = 1 \}.
\end{align*}
Using these sets, a new way to express $\Omega_l$ is derived:
\begin{equation*}
    \Omega_l = \{ \mathbf{w}_l \in \mathbb{R}^{p_l}; \quad \mathbf{w}_l = \mathbf{W}_l \boldsymbol{\lambda}_l; \quad \mathbf{W}_l \in \Omega_\text{mat} \cap \Omega_\text{orth}; \quad \boldsymbol{\lambda}_l \in \Lambda_l \}
\end{equation*}
Therefore, $\Omega_l$ is the image of the set $\Lambda_l \times (\Omega_\text{mat} \cap \Omega_\text{orth})$ by the continuous application $f:(\boldsymbol{\lambda}_l, \mathbf{W}_l) \mapsto \mathbf{W}_l \boldsymbol{\lambda}_l$. The proof that $\Omega_l$ is compact then reduces to prove that $\Lambda_l$ and $\Omega_\text{mat} \cap \Omega_\text{orth}$ are compact.

$\Lambda_l$ is compact as the boundary of the norm 2 unit ball in $\mathbb{R}^{R_l}$ which is of finite dimension.

We will now show that $\Omega_\text{mat} \cap \Omega_\text{orth}$ is compact as the intersection of a compact set with a closed set.
\begin{itemize}
    \item $\Omega_\text{norm}$ is a compact set as the boundary of the unit ball of the norm induced by the scalar product $\langle \cdot | \cdot \rangle: (\mathbf{x}, \mathbf{y}) \mapsto \mathbf{x}^\top \mathbf{M}_l \mathbf{y}$ where $\mathbf{M}_l$ is symmetric positive-definite.
    \item $\Omega_\text{kron}$ is a closed set. It is a standard result in geometric algebra and a specificity of the set of rank-1 tensors. 
    %It does not hold in the general case with arbitrary rank and order. 
    \item $\Omega_\text{norm} \cap \Omega_\text{kron}$ is compact as the intersection of a closed and a compact set.
    \item $\Omega_\text{mat}$ is the image of $\times_{R_l}(\Omega_\text{norm} \cap \Omega_\text{kron})$ (the Cartesian product $R_l$ times) by the continuous operator that arranges vectors into a matrix. Hence, $\Omega_\text{mat}$ is compact. 
    \item $\Omega_\text{orth}$ is the set of semi-orthogonal matrices. This set is closed (and even compact but we only need it to be closed).
\end{itemize}
Consequently, $\Omega_\text{mat} \cap \Omega_\text{orth}$ is compact and we have shown that $\Omega_l$ is a compact set.

This demonstration is suited in the non-separable case. A slightly different demonstration can be developed in the separable one, where two different versions of $\Omega_{\text{orth}}$ are preferred. One for the strong orthogonal case, where $\Omega_{\text{orth}}^{v} = \times_{d_l} \Omega_{\text{orth}}^{v, m}$, with $\Omega_{\text{orth}}^{v, m} = \lbrace \mathbf{V}_{l,m} \in \mathbb{R}^{p_{l,m} \times R_l}; \quad \mathbf{V}_{l,m}^\top  \mathbf{V}_{l,m} = \mathbf{I}_{R_l}\rbrace$. One for the case where only one mode $m$ bears the orthogonality, with $\Omega_{\text{orth}}^{v} = \Omega_{\text{norm}}^{v, 1} \times \ldots \times \Omega_{\text{orth}}^{v, m} \times \ldots \times \Omega_{\text{norm}}^{v, d_l}$, where $\Omega_{\text{norm}}^{v, q} = \lbrace \mathbf{V}_{l,q} \in \mathbb{R}^{p_{l,q} \times R_l}; \quad \Vert \mathbf{v}_{l,q}^{(r)} \Vert_2^2 = 1, r\in\left[R\right]\rbrace$. Similar arguments can be derived to show that $\Omega_l^v$ is indeed compact.

\subsection{Update for non-separable TGCCA}
\label{general-update}
The goal is still to solve the optimization problem of TGCCA stated in \eqref{TGCCA}, but this time, without any separable assumptions made on matrices $\mathbf M_l, l \in [L]$ used in the constraint sets $\Omega_l, l \in [L]$. This makes this non-separable TGCCA more general as it can handle positive definite matrices $\mathbf M_l$ of any type. However, at the level of the constraints, it also entangles the rank factors inside a single-mode. Thus, as
opposed to the separable case, we alternate between the $\mathbf w_{l, m}^{(r)}$ for $m \in [d_l]$ and $r \in [R_l]$ instead of finding all $\{\mathbf w_{l,m}^{(r)}\}_{r \in [R_l]}$ at once for a given $m$ to find an update for the non-separable case. 

We start by rewriting the constraints on $\mathbf w_l^{(r)}$ in terms of $\mathbf w_{l,m}^{(r)}$. Using the same trick as in paragraph \ref{sample_sep_TGCCA}, $\mathbf w_l^{(r)} = \mathbf W_{l, (-m)}^{(r)} \mathbf w_{l, m}^{(r)}$ with $\mathbf{W}_{l, (-m)}^{(r)} = \left( \mathbf{w}_{l,d_l}^{(r)} \otimes \dots \otimes \mathbf{w}_{l, m+1}^{(r)} \otimes \mathbf{I}_{p_{l,m}} \otimes \mathbf{w}_{l, m-1}^{(r)} \otimes \dots \otimes \mathbf{w}_{l,1}^{(r)} \right) \in \mathbb{R}^{p_l \times p_{l,m}}$. We further introduce the matrix $\Mr = \mathbf W_{l, (-m)}^{(r) \top} \hat{\mathbf M}_l \mathbf W_{l, (-m)}^{(r)} \in \mathbb{R}^{p_{l,m} \times p_{l,m}}$ that we assume to be invertible. Hence the previous constraints
\begin{equation*}
    \left\{
    \begin{array}{ll}
            \mathbf w_l^{(r) \top} \hat{\mathbf M}_l \mathbf w_l^{(r)} = 1 \\
            \mathbf w_l^{(r) \top} \hat{\mathbf M}_l \mathbf w_l^{(s)} = 0 \quad \text{for } r \neq s,
        \end{array}
    \right.
\end{equation*}
now read
\begin{equation*}
    \left\{
    \begin{array}{ll}
            \mathbf w_{l,m}^{(r) \top} \Mr \mathbf w_{l,m}^{(r)} = 1 \\
            \mathbf w_{l,m}^{(r) \top} \mathbf W_{l, (-m)}^{(r) \top} \hat{\mathbf M}_l \mathbf w_l^{(s)} = 0 \quad \text{for } r \neq s.
        \end{array}
    \right.
\end{equation*}
The Lagrangian associated with the considered optimisation problem is then 
\begin{align}
    \mathcal{L}(\mathbf{w}_{l,m}^{(r)}, \nu, \boldsymbol{\mu}) = - \lambda_l^{(r)} \nabla_l f(\mathbf{w})^\top \mathbf{W}_{l, (-m)}^{(r)} \mathbf{w}_{l,m}^{(r)} &+ \frac{1}{2} \nu (\mathbf{w}_{l,m}^{(r) \top} \Mr \mathbf{w}_{l,m}^{(r)} - 1) \nonumber \\
    &+ \mathbf{w}_{l,m}^{(r) \top} \mathbf{W}_{l, (-m)}^{(r) \top} \hat{\mathbf{M}}_l \mathbf{W}_l^{(-r)} \boldsymbol{\mu} ,
\end{align}
where $ \mathbf{W}_l^{(-r)} = \begin{bmatrix} \mathbf{w}_l^{(1)} & \dots & \mathbf{w}_l^{(r - 1)} & \mathbf{w}_l^{(r + 1)} & \dots & \mathbf{w}_l^{(R_l)} \end{bmatrix} \in \mathbb{R}^{p_l \times (R_l - 1)}$. The computations are a bit cumbersome, but there is no real difficulty here. The following derivations lead to a closed-form solution of the Lagrangian.

Canceling the derivatives of the Lagrangian function with respect to $\mathbf{w}_{l,m}^{(r)}$, $\nu$ and $\boldsymbol{\mu}$ yields the following stationary equations:
\begin{align}
    &\hat{\nu} ~ \hat{\mathbf{w}}_{l,m}^{(r)} = \left( \Mr \right)^{-1} \mathbf{W}_{l, (-m)}^{(r)^\top} \left( \lambda_l^{(r)}  \nabla_l f(\mathbf{w}) - \hat{\mathbf{M}}_l \mathbf{W}_l^{(-r)} \hat{\boldsymbol{\mu}} \right)   \label{1} \\
    &\hat{\mathbf{w}}_{l,m}^{(r)\top} \Mr \hat{\mathbf{w}}_{l,m}^{(r)} = 1 \label{2} \\
    &\mathbf{W}_l^{(-r)\top} \hat{\mathbf{M}}_l \mathbf{W}_{l, (-m)}^{(r)} \hat{\mathbf{w}}_{l,m}^{(r)} = 0.
    \label{3}
\end{align}

We start by playing with the equations to isolate $\hat{\boldsymbol \mu}$. Left multiplying \eqref{1} by $\mathbf{W}_l^{(-r) \top} \hat{\mathbf{M}}_l \mathbf{W}_{l, (-m)}^{(r)}$ and using \eqref{3} we get:
\begin{equation}
    \mathbf{W}_l^{(-r) \top} \hat{\mathbf{M}}_l \mathbf{W}_{l, (-m)}^{(r)} \left( \Mr \right)^{-1} \mathbf{W}_{l, (-m)}^{(r)^\top} \left( \lambda_l^{(r)}  \nabla_l f(\mathbf{w}) - \hat{\mathbf{M}}_l \mathbf{W}_l^{(-r)} \hat{\boldsymbol{\mu}} \right) = 0. \label{eq:mu_intermediary}
\end{equation}

We introduce $\mathbf Z =  \left( \Mr \right)^{-1/2} \mathbf{W}_{l, (-m)}^{(r)^\top} \hat{\mathbf{M}}_l \mathbf{W}_l^{(-r)} \in \mathbb{R}^{p_{l, m} \times (R_l - 1)}$, this allows us to rewrite the previous equation as
\begin{equation*}
    \mathbf{Z}^\top \mathbf{Z}\hat{\boldsymbol{\mu}} = \lambda_l^{(r)} \mathbf{Z}^\top \left( \Mr \right)^{-1/2} \mathbf{W}_{l, (-m)}^{(r)^\top} \nabla_l f(\mathbf{w}).
\end{equation*}
Assuming that $\mathbf Z$ has full rank, we can isolate $\hat{\boldsymbol \mu}$:
\begin{equation}
    \hat{\boldsymbol{\mu}} = \lambda_l^{(r)} \left( \mathbf{Z}^\top \mathbf{Z} \right)^{-1} \mathbf{Z}^\top \left( \Mr \right)^{-1/2} \mathbf{W}_{l, (-m)}^{(r)^\top} \nabla_l f(\mathbf{w}). \label{eq:mu_formula}
\end{equation}
We will now find the value of $\hat{\nu}$. From equation (\ref{eq:mu_formula}), we can rewrite (\ref{1}) as
\begin{eqnarray}
    \hat{\nu} ~ \hat{\mathbf{w}}_{l,m}^{(r)} =& \left( \Mr \right)^{-1/2} &\left[ \lambda_l^{(r)} \left( \Mr \right)^{-1/2}\mathbf{W}_{l, (-m)}^{(r)^\top}  \nabla_l f(\mathbf{w})\right. \nonumber \\ 
    && ~ - \left.\lambda_l^{(r)} \mathbf{Z} \left( \mathbf{Z}^\top \mathbf{Z} \right)^{-1} \mathbf{Z}^\top \left( \Mr \right)^{-1/2} \mathbf{W}_{l, (-m)}^{(r)^\top} \nabla_l f(\mathbf{w})\right] \nonumber\\
     =&\lambda_l^{(r)} \left( \Mr \right)^{-1/2}&\left( \mathbf{I} - \Pimr \right) \left( \Mr \right)^{-1/2} \mathbf{W}_{l, (-m)}^{(r)^\top} \nabla_l f(\mathbf{w}), \label{eq:w_intermediary}
\end{eqnarray}
with $\Pimr \equiv \mathbf{Z}  \left( \mathbf{Z}^{\top} \mathbf{Z} \right)^{-1} \mathbf{Z}^\top$ the orthogonal projector on the space spanned by $\mathbf{Z}$. We can now combine \eqref{1}, \eqref{2} and \eqref{eq:w_intermediary} to find the value of $\hat{\nu}$:
\begin{equation}
    \hat{\nu} = |\lambda_l^{(r)}| \sqrt{ \nabla_l f(\mathbf{w})^\top \mathbf{W}_{l, (-m)}^{(r)} \left( \Mr \right)^{-1/2} \left( \mathbf{I} - \Pimr \right) \left( \Mr \right)^{-1/2} \mathbf{W}_{l, (-m)}^{(r)^\top} \nabla_l f(\mathbf{w}) }.
\end{equation}
Finally, assuming that $\hat{\nu}$ is not null, we find $\hat{\mathbf{w}}_{l,m}^{(r)}$:
\begin{equation}
    \hat{\mathbf{w}}_{l,m}^{(r)} = \frac{\text{sign}\left( \lambda_l^{(r)} \right)
        \left( \Mr \right)^{-1/2} \left( \mathbf{I} - \Pimr \right) \left( \Mr \right)^{-1/2} \mathbf{W}_{l, (-m)}^{(r)^\top} \nabla_l f(\mathbf{w})
    }{
        \sqrt{\nabla_l f(\mathbf{w})^\top \mathbf{W}_{l, (-m)}^{(r)} \left( \Mr \right)^{-1/2} \left( \mathbf{I} - \Pimr \right) \left( \Mr \right)^{-1/2} \mathbf{W}_{l, (-m)}^{(r)^\top} \nabla_l f(\mathbf{w}) }
    }.
\end{equation}

\subsection{Uniqueness of the update for non-separable TGCCA}
We come back on some of the assumptions we made during the derivation of $\hat{\mathbf{w}}_{l,m}^{(r)}$. We first assumed that $\mathbf Z$ had full rank. Sometimes, complete rows of $\mathbf{W}_{l}^{(-r)^\top} \hat{\mathbf{M}}_l \mathbf{W}_{l, (-m)}^{(r)}$ are equal to $0$. It means that whatever the choice of $\mathbf{w}_{l,m}^{(r)}$, $\mathbf{w}_{l}^{(r)}$ is orthogonal to the corresponding rows, so to the corresponding rank-1 factors. 
\iffalse
For example when $\hat{\mathbf{M}}_l = \hat{\mathbf{M}}_{l,d_l} \otimes \dots \otimes \hat{\mathbf{M}}_{l,1}$, the  $s^\text{th}$ row of $\mathbf{W}_{l}^{(-r)^\top} \hat{\mathbf{M}}_l \mathbf{W}_{l, (-m)}^{(r)}$, associated with the orthogonality constraint with respect to the $s^\text{th}$ rank-1 factor, can be written as 
    \begin{equation*}
        \mathbf{w}_{l}^{(s)^\top}\hat{\mathbf{M}}_l \mathbf{W}_{l, (-m)}^{(r)} = \left( \mathbf{w}_{l, d_l}^{(s)^\top}\hat{\mathbf{M}}_{l,d_l}\mathbf{w}_{l, d_l}^{(r)} \right)\times \ldots \times \left( \mathbf{w}_{l, 1}^{(s)^\top}\hat{\mathbf{M}}_{l,1}\mathbf{w}_{l, 1}^{(r)} \right) \mathbf{w}_{l, m}^{(s)^\top}\hat{\mathbf{M}}_{l,m}.
    \end{equation*}
Thus, the orthogonality can be handled by a single mode. 
\fi
We can define $\mathcal{I}_r$ as the set of indices of factors to which $\mathbf{w}_{l}^{(r)}$ is already orthogonal whatever the choice for $\mathbf{w}_{l,m}^{(r)}$. Using the complementary conditions, it means that $\mathbf{\mu}_i = 0, ~ \forall i \in \mathcal{I}_r$. Finally, the same expressions can be derived in order to solve (\ref{update}) by replacing $\mathbf{W}_l^{(-r)}$ with $\mathbf{W}_l^{(-r, -\mathcal{I}_r)}$, which is similar to $\mathbf{W}_l^{(-r)}$ but with all columns with their indices in $\mathcal{I}_r$ that are also removed. The extreme case being when all indices (except $r$) are in $\mathcal{I}_r$. In this situation, it can be shown that 
    \begin{equation*}
        \hat{\mathbf{w}}_{l,m}^{(r)} = \frac{\text{sign}\left( \lambda_l^{(r)} \right)
        \left( \Mr \right)^{-1} \mathbf{W}_{l, (-m)}^{(r)^\top} \nabla_l f(\mathbf{w})
    }{
        \sqrt{\nabla_l f(\mathbf{w})^\top \mathbf{W}_{l, (-m)}^{(r)} \left( \Mr \right)^{-1} \mathbf{W}_{l, (-m)}^{(r)^\top} \nabla_l f(\mathbf{w}) }
    }.
    \end{equation*}
    However, even if we remove columns of $\mathbf{W}_l^{(-r)}$, there may be some configurations where $\mathbf{Z}$ does not have full rank. We did not witness such configuration in practice and $\mathbf{Z} \in \mathbb{R}^{p_{l, m} \times R_l^*}$ where $R_l^*$ is at most $R_l - 1$. We advise to choose $R_l$ small compared to $p_{l, m}$. 
    
We later assumed that $\hat{\nu}$ was not null. If $\hat{\nu} = 0$, equation (\ref{eq:mu_intermediary}) and thus (\ref{eq:mu_formula}) and (\ref{eq:w_intermediary}) still hold. Now, as $\hat{\nu} = 0$, if $\lambda_l^{(r)} \neq 0$, (\ref{eq:w_intermediary}) can be rewritten as
    \begin{equation*}
        \left( \mathbf{I} - \Pimr \right) \left( \Mr \right)^{-1/2} \mathbf{W}_{l, (-m)}^{(r)^\top} \nabla_l f(\mathbf{w}) = 0,
    \end{equation*}
    which means that $\left( \Mr \right)^{-1/2} \mathbf{W}_{l, (-m)}^{(r)^\top} \nabla_l f(\mathbf{w})$ is in the linear space spanned by $\mathbf{Z}$ and so that $\mathbf{W}_{l, (-m)}^{(r)^\top} \nabla_l f(\mathbf{w})$ is in the linear space spanned by $\mathbf{W}_{l, (-m)}^{(r)^\top} \hat{\mathbf{M}}_l \mathbf{W}_l^{(-r)}$. 
    This last assertion and the fact that, for any $\mathbf{w}_{l,m}^{(r)}$ satisfying the constraints, equation \eqref{3} is verified, yield  $\mathbf{w}_{l,m}^{(r)^\top}\mathbf{W}_{l, (-m)}^{(r)^\top} \nabla_l f(\mathbf{w}) = 0$. 
    Thus, the maximum value for (\ref{update}) is $0$ and is reached for any $\mathbf{w}_{l,m}^{(r)}$.
    
    If $\lambda_l^{(r)} = 0$, as $\lambda_l^{(r)}$ is the weight of the term $\mathbf{w}_l^{(r)}$, it means that the maximum value for (\ref{update}) is $0$ and is reached for any $\mathbf{w}_{l}^{(r)}$.  In both cases, a solution is to not update $\mathbf{w}_{l,m}^{(r)}$, this preserves the uniqueness of the global update $\text{r}_l(\mathbf{w})$.
    
\subsection{Limitations of non-separable TGCCA}
The simulations show that non-separable TGCCA is slow and does not perform as well as separable TGCCA when $R_l > 1$, even when the separable assumption is wrong. The speed issue is related to the fact that, for each update, we invert a matrix of size $p_{l,m} \times p_{l,m}$, which can be rather big. The performance issue is probably due to the fact that, by alternating on the $\mathbf w_{l,m}^{(r)}$ for $r \in [R_l]$ and $m \in [d_l]$, the constraints are no longer separable, and modifying one vector $\mathbf w_{l,m}^{(r)}$ changes the constraint on another vector $\mathbf w_{l,m}^{(s)}$. 
This kind of behavior tends to make alternate algorithms get stuck on points on the border of the feasible sets, which are away from optima. An attractive solution would be to directly find an update of $\mathbf W_{l,m}$, like in the case of separable TGCCA. This direction is currently being investigated.
